# Supplementary material for: Benchmarking Large Language Models for Molecule Prediction Tasks
Source: arXiv:2403.05075 source file (2024-03-08)
Supplement: Supplementary file 1 [file appendix_prompt.tex]

\textbf{Input-Feature (IF)}.
Asking LLMs to extract helpful knowledge for given tasks based on natural language description of the tasks.
\begin{regbox} \textit{\textbf{IF Prompt Example}}
\begin{verbatim}
<Instruction>
Provide helpful information to predict if the Target molecule inhibits HIV virus 
replication.
</Instruction> 
<Target>
Molecule: Oc1ccc(Cl)cc1C(c1cc(Cl)ccc1O)C(Cl)(Cl)Cl. 
Caption: The molecule is a quaternary ammonium... 
</Target> 
Answer:
\end{verbatim}
\end{regbox}

\textbf{Input-Prediction (IP)}~\cite{BMRS20}.
Asking LLMs to make predictions for given tasks based on natural language description of the tasks.
\begin{regbox} \textit{\textbf{IP Prompt Example}}
\begin{verbatim}
<Instruction> 
Predict if the Target molecule inhibits HIV virus replication. Use this format: 
Prediction: <number, 1 means target molecule inhibits HIV virus replication, 0 means 
target molecule does not inhibit HIV virus replication>; 
</Instruction> 
<Target>
Molecule Oc1ccc(Cl)cc1C(c1cc(Cl)ccc1O)C(Cl)(Cl)Cl. 
Caption: The molecule is a quaternary ammonium... 
</Target> 
Answer: 
\end{verbatim}
\end{regbox}

\textbf{Input-Explanation (IE)}~\cite{HBLH23}.
Inspired by \cite{HBLH23}, which leverages LLM generated explanations to boost GNN performance on ordinary tasks, we propose our EP template. 
\begin{regbox} \textit{\textbf{\IE Prompt Example}}
\begin{verbatim}
<Instruction>
Predict if the Target molecule is HIV activate, and provide explanations. Use this
format:
Prediction: <number, 1 means target molecule is HIV activate, 0 means target molecule 
is not HIV activate>
Explanation: <sentence>
</Instruction>
<Target>
Molecule Oc1ccc(Cl)cc1C(c1cc(Cl)ccc1O)C(Cl)(Cl)Cl.
Caption: The molecule is a quaternary ammonium...
</Target>
Answer:
\end{verbatim}
\end{regbox}

\textbf{Few-shot (FS)}~\cite{WWSBIXCLZ22}.
A few demonstrations are given to LLMs, as task-related knowledge, to export more helpful task-specific knowledge. 
\begin{regbox} \textit{\textbf{FS Prompt Example}}
\begin{verbatim}
<Knowledge>
Try to use the provided Knowledge whenever possible:
The label of Molecule O=Nc1ccc(O)c(N=O)c1O is 1;
The label of Molecule Nc1ccc(C=Cc2ccc(N)cc2S(=O)(=O)O)c(S(=O)(=O)O)c1 is 0;
...
</Knowledge>
<Instruction>
Predict if the Target molecule is HIV activate or not, and provide explanations. Use 
this format:
Prediction: <number, 1 means target molecule is HIV activate, 0 means target molecule 
is not HIV activate>
Explanation: <sentence>
</Instruction>
<Target>
Molecule Oc1ccc(Cl)cc1C(c1cc(Cl)ccc1O)C(Cl)(Cl)Cl.
Caption: The molecule is a quaternary ammonium...
</Target>
Answer:
\end{verbatim}
\end{regbox}
