# Supplementary material for: Benchmarking Large Language Models for Molecule Prediction Tasks
Source: arXiv:2403.05075 source file (2024-03-08)
Supplement: Supplementary file 2 [file appendix_experiment.tex]

\input{tables/table-complete-performance}
